# Supplementary material for: Causality-Enhanced Behavior Sequence Modeling in LLMs for Personalized Recommendation
Source: arXiv:2410.22809 source file (2024-10-30)
Supplement: Supplementary file 1 [file 8_appendix.tex]

\section{Hyper-parameter Analysis} 
We use BIGRec+CFT on the Book dataset as an example to examine the influence of two key hyper-parameters in our methods: 1) $\lambda$ in Equation~\eqref{eq:multitask}, which controls the weight of the new task loss, and 2) $\beta$ in Equation~\eqref{eq:weighting}, which regulates the weight for the last token. To isolate the effects of each hyper-parameter, we kept the other fixed during our study. 
Figure~\ref{fig:hyper} summarizes the results. For $\lambda$, we explore a narrow range of similar scales. As shown in the figure, CFT is sensitive to $\lambda$—even a slight increase can cause the method to crash, as higher values often lead to the model generating garbled text across all datasets. Therefore, it is better to tune it starting from relatively small values (e.g., 0.01, 0.02). For $\beta$, we investigate a broader range. The figure indicates that the model generally performs better at either the highest or lowest values, suggesting that when tuning $\beta$, it is advisable to start with the extremes before adjusting toward the middle range.
\begin{figure}[h]
\centering

% \subfigure[\textbf{$\beta$ = 1 - 1/1.2}]
\subfigure
{\includegraphics[width=0.23\textwidth]{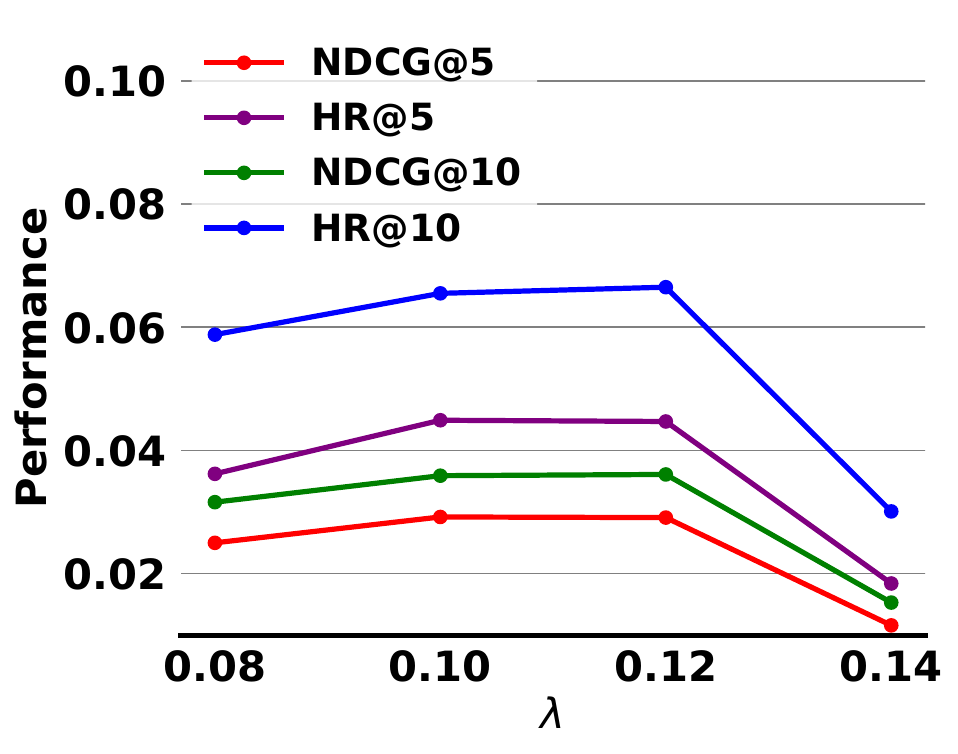}}
% \subfigure[ \textbf{$\lambda$ = 0.10}]
\subfigure
{\includegraphics[width=0.23\textwidth]{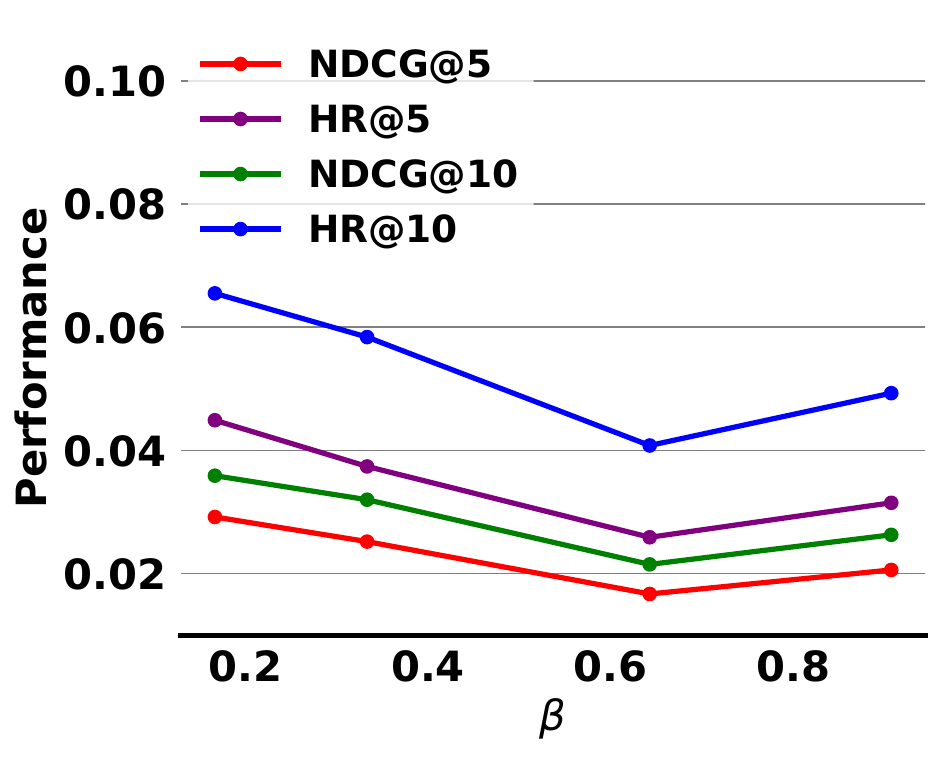}}
% \quad
% \vspace{-15pt}
\caption{Performance comparison of varying hyper-parameters on Books dataset. The left side represents the result of $\lambda$ and the right side represents the result of $\beta$.}
\label{fig:hyper}
\vspace{-10pt}
\Description{..}
\end{figure}

% \section{Recommend Analysis on CDs}

% \begin{figure}[t]
% \centering
% \subfigure[ \textbf{CDs With History}]{ \includegraphics[width=0.23\textwidth]{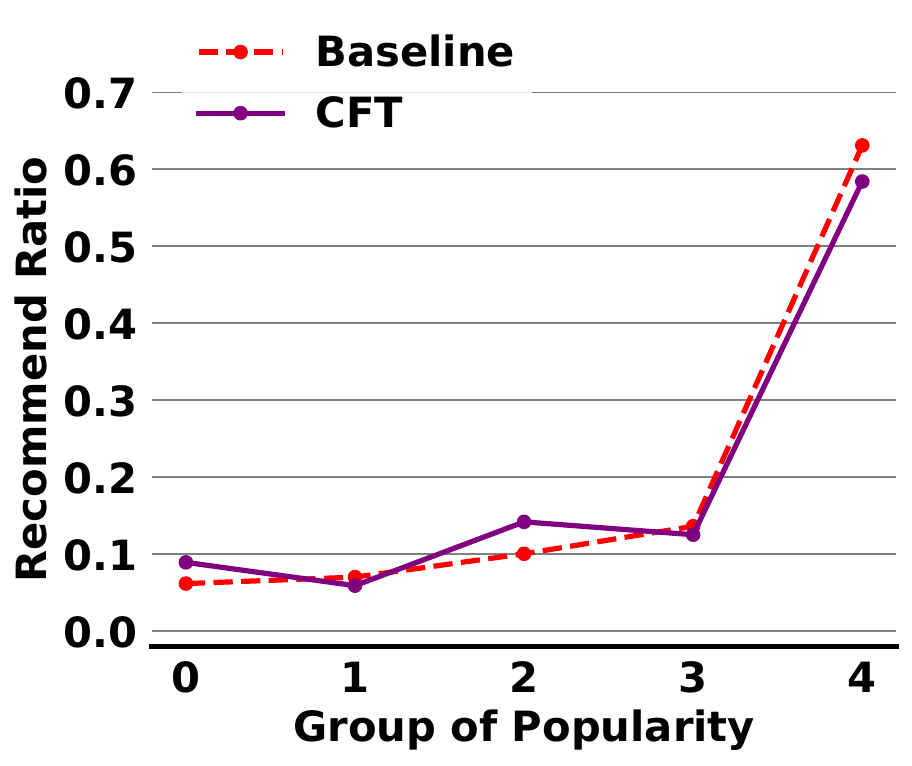}}
% \subfigure[ \textbf{CDs Without History}]{ \includegraphics[width=0.23\textwidth]{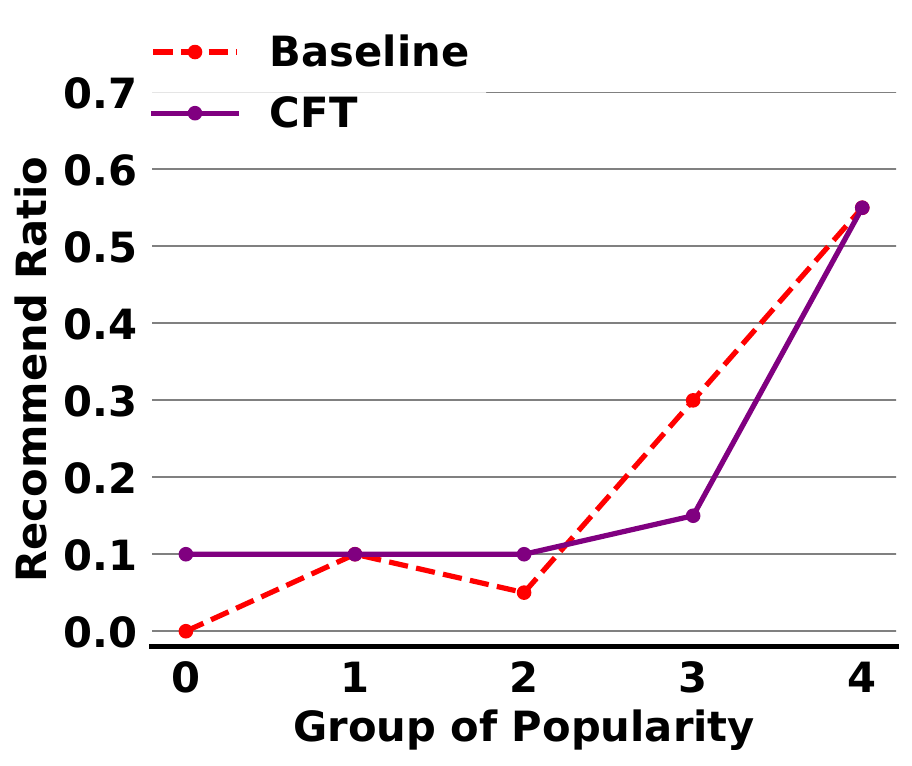}}
% \caption{Top-20 recommendation distribution comparison between BIGRec (Baseline) and BIGRec + CFT (CFT).}
% \label{fig:cmp-cft}
% \end{figure}
